# Supplementary material for: Provable Privacy with Non-Private Pre-Processing
Source: arXiv:2403.13041 source file (2024-06-21)
Supplement: Supplementary file 1 [file app.tex]

\section{Lemmas}

\begin{lem}[Upper bound on memorization by DP]
Define the leave one out accuracy of an algorithm for a dataset $S$ and a sample $x\in S$ as $\LOOAcc(\cA, S, x) = \bP_{h\sim \cA(S\setminus \{x\}}(h(x) = y)$. If $\cA$ is $(\epsilon, \delta)$-DP, then for any $S\in \cX^n$ and $x\in S$, 
\[mem(\cA, S, x) \leq \LOOAcc(\cA, S, x) (e^\epsilon + \delta - 1). \]
\end{lem}

\begin{proof}
    By definition of DP, let $O$ be the set of hypothesis $h$ that correctly classifies the point $x$, i.e. $O = \{h\in \cH: h(x) = y\}$. Then, 
    \[\frac{\bP_{h\sim \cA(S)}[h(x) = y]}{\bP_{h\sim \cA(S\setminus \{x\})}[h(x) = y]} = \frac{\bP[\cA(S) \in O]}{\bP[\cA(S\setminus \{x\}) \in O]}\leq \max_{S, S', O\in \cY}\frac{\bP[\cA(S) \in O]}{\bP[\cA(S\setminus \{x\}) \in O]}\leq e^\epsilon + \delta. \]
    The upper bound on memorization follows by rearranging the above the inequality, \[\bP_{h\sim \cA(S)}[h(x) = y]\leq (e^\epsilon + \delta)\LOOAcc(\cA, S, x). \]
\end{proof}

\section{data deduplication}
We consider the approximate label-independent data-deduplication algorithm similar to \cite{debenedetti2023privacy}, \ie two data points $(x_i, y_i), (x_j, y_j)$ satisfying $\norm{x_i - x_j}_2 < \delta$ are approximate duplicates regardless of their labels. The data deduplication algorithm $\pi$ replaces all duplicates with one point in the set of approximate duplicates uniformly at random. 

Consider the following regularized objective perturbation algorithm from DP-ERM, 

\begin{algorithm}
\caption{Regularized Objective Perturbation }
\textbf{Input}: Dataset $S = \{(x_1, y_1), \ldots (x_n, y_n)\}$, privacy parameter $\epsilon$, Regularization parameter $\Lambda$, parameters of the loss function $c_1, c_2$. 
\begin{algorithmic}[1]
    \State Let $\epsilon' = \epsilon - \log \br{1 + \frac{2c_1}{n\Lambda} + \frac{c_1^2}{n^2\Lambda^2}}$
    \State If $\epsilon' > 0$, then $\Delta = 0$, else $\Delta = \frac{c_1}{(e^{\epsilon/4})} - \Lambda$, and $\epsilon' = \epsilon / 2$. 
    \State Draw a vector $b\propto e^{-\frac{\epsilon'\norm{b}_2}{2}}$
    \State Output \begin{equation}\label{eq:output-perturbation-optimization}
        \hat{w} = \argmin_w \frac{1}{n}\sum_{i = 1}^n \ell(w; (x_i, y_i)) + \frac{\Lambda + \Delta}{2}\norm{w}_2^2 + \frac{1}{n}b^\top w
    \end{equation}
\end{algorithmic}
\end{algorithm}

\begin{thm}\label{thm:deduplication}
    For the label independent data-deduplication algorithm $\pi$ defined above, let $\cA$ be objective perturbation with regularized cross-entropy loss $L(w; S) = \frac{1}{n}\sum_{i = 1}^n \ell(w; (x_i, y_i)) + \frac{\lambda}{2}\norm{w}_2^2$ with $c = 1/4$. Then, $\cA$ is $(\epsilon, 0)$-DP on deduplicated data and 
    \[
    \max_{S, S', o}\log\br{\frac{\bP\bs{\cA(\pi(S)) \in o}}{\bP\bs{\cA(\pi(S')) \in o}}}\geq \Omega( n \epsilon) 
    \]
    with probability $1/n$. 
\end{thm}

\begin{proof}
    Let $S_1 = \{(x_1, -1), \ldots, (x_{n/2}, -1), (x_{(n/2 + 1)}, 1), \ldots, (x', 1)\}$ where for all $i \geq n/2 + 1$, $\norm{x_i - x'} \leq \delta$. Let $S_2=\{(x_1, -1), \ldots, (x_{n/2}, -1), (x_{(n/2 + 1)}, 1), \ldots, (x', -1)\}$ differing from $S_1$ at the last point. 

    By the definition of the data deduplication algorithm $\pi$, with probability $4/n^2$, $S_1' = \pi(S_1) = \{(x_1, -1), \ldots, (x', 1), \ldots, (x', 1)\}$ and $\pi(S_2) = S_2' = \{(x_1, -1), \ldots, (x', -1), \ldots, (x', -1)\}$. 

    For regularized output perturbation described above, the exact solution to the optimization problem in~\Cref{eq:output-perturbation-optimization} induces a one-to-one relationship between the output $w$ and the random vector $b_S$ for a fixed dataset $S$ by setting the first derivative of~\Cref{eq:output-perturbation-optimization} to $0$,
    \begin{equation}
        \label{eq:one-to-one-function-w-to-b}
        b_S = -n(\Lambda + \Delta) w - \sum_{i = 1}^n y_i \ell'(y_iw^\top x_i) x_i =: f(w; S)
    \end{equation}
    
    For any $w\in B_2^d$, \begin{equation}
    \begin{aligned}
            \frac{\bP[\cA(\pi(S_1)) = w]}{\bP[\cA(\pi(S_2)) = w]}
            &=         \frac{\bP[\cA(S_1') = w]}{\bP[\cA(S_2') = w]}\\
            &= \frac{\bP[b = f(w, S_1')]\abs{\text{det}(\nabla_w f(w; S_1'))}^{-1}}{\bP[b = f(w, S_2')]\abs{\text{det}(\nabla_w f(w; S_2'))}^{-1}} 
    \end{aligned}
    \end{equation}
    Next, we will lower bound $\frac{\bP[b = f(w, S_1')]}{\bP[b = f(w, S_2')]}$ and $\frac{\abs{\text{det}(\nabla_w f(w; S_1'))}^{-1}}{\abs{\text{det}(\nabla_w f(w; S_2'))}^{-1}} $ separately. 
    \begin{equation}
        \begin{aligned}
            \frac{\bP[b = f(w, S_1')]}{\bP[b = f(w, S_2')]} 
            =& e^{\frac{\epsilon'}{2}\br{\norm{f(w; S_2')}^2 - \norm{f(w; S_1')}^2}}\\
            =& e^{\frac{\epsilon'}{2}\br{(f_1 + f_2)^\top (f_1 - f_2)}}\\
           =& \exp\frac{\epsilon'}{2}\br{-2(\Lambda + \Delta)w + 2\sum_{i = 1}^{n/2} \ell'(-w^\top x_i)x_i + \sum_{i = n/2+1}^n \br{\ell'(-w^\top x_i) - \ell'(w^\top x_i)}x_i}\\
            &\br{-\sum_{i = n/2 + 1}^n \br{\ell'(w^\top x_i) + \ell'(-w^\top x_i)}x_i}\\
            \overset{(a)}{=}& \exp\br{-2(\Lambda + \Delta)w + 2\sum_{i = 1}^{n/2} \ell'(-w^\top x_i)x_i + \sum_{i = n/2+1}^n x_i}\br{\sum_{i = n/2 + 1}^n x_i}\\
            =& \exp\br{\frac{\epsilon'}{2}\br{c_1w^\top 
 +c_2^\top X}X^\top c_3}\\
 \overset{(b)}{\geq}& \exp\br{\epsilon' n\br{\lambda_n(XX^\top) - (\Lambda + \Delta)}}
        \end{aligned}
    \end{equation}
where step (a) follows from $\ell'(z) - \ell'(-z) = 1$ and $\ell'(z) + \ell'(-z) = -1$ for logistic loss function $\ell(z) = \log(1+e^{-z})$ with $\ell'(z) = \frac{-1}{1+e^z}$, and $c_1 := -2(\Lambda + \Delta)$, $c_2 := [2\ell'(-w^\top x_1), \ldots, 2\ell'(-w^\top x_{n/2}), 1, \ldots, 1]^\top $, $c_3 := [0, \ldots, 0, 1, \ldots, 1]^\top$. Step (b) follows as $\lambda_d(XX^\top)$ is the smallest eigenvalue of $XX^\top$. 

For $\norm{\tilde{z}-z}\leq \delta$, we can apply Taylor expansion on $\ell'$ and obtain similar results, \begin{equation}
    \ell'(\tilde{z}) - \ell'(z) \approx \ell'(z) + \br{\tilde{z} - z}\ell''(z) - \ell'(-z) \in\br{ (1-0.3\delta), (1+0.3\delta)} 
\end{equation} 
where the second inequality follows from $\ell''(z) \leq 0.3$ for all $z\in \reals$. 
Similarly, 
\begin{equation}
    \ell'(\tilde{z}) + \ell'(z) \approx \ell'(z) + \br{\tilde{z} - z}\ell''(z) + \ell'(-z) \in\br{ (-1-0.3\delta), (-1+0.3\delta)}
\end{equation}
\begin{equation}
        \nabla_w f(w, S) = -n(\Lambda + \Delta) I_d - \sum_{i = 1}^n y_i^2 \ell''(y_i w^\top x_i) x_i x_i^\top 
\end{equation}

\begin{equation}\label{eq:det-def}
    \begin{aligned}
        \det\br{\nabla_w f(w; S_1')} &= -\det\br{n(\Lambda + \Delta) I_d + \sum_{i = 1}^n y_i^2 \ell''(y_i w^\top x_i) x_i x_i^\top }\\
        &=- \det\br{n(\Lambda + \Delta)I_d + \sum_{i = 1}^{n-1} y_i^2 \ell''(y_i w^\top x_i) x_i x_i^\top + y_n^2 \ell''(y_n w^\top x_n) x_n x_n^\top }
    \end{aligned}
\end{equation}
Write $A_j = n(\Lambda + \Delta)I_d + \sum_{i = 1}^{j} y_i^2 \ell''(y_i w^\top x_i) x_i x_i^\top $ with $A_0 =n(\Lambda + \Delta)I_d $, we apply~\Cref{lem:matrix-determinant-lemma} to~\Cref{eq:det-def} recursively, 
\begin{equation}
    \label{eq:det-deriv}
    \begin{aligned}
        \det\br{\nabla_w f(w; S_1')} &= -\det\br{A_{n-1}}\br{1 + y_n^2 \ell''(y_n w^\top x_n)x_n^\top A_{n-1}^{-1}x_n}\\
        &= -\det \br{A_{n-1}}\br{1 + y_{n-1}^2 \ell''(y_{n-1} w^\top x_{n-1})x_{n-1}^\top A_{n-2}^{-1}x_{n-1}}\br{1 + y_n^2 \ell''(y_n w^\top x_n)x_n^\top A_{n-1}^{-1}x_n}\\
        &= \ldots \\
        &= -\det \br{n(\Lambda + \Delta)I_d}\prod_{i = 1}^n \br{1 + y_i^2 \ell''(y_i w^\top x_i)x_i^\top A_{i-1}^{-1}x_i}\\
        &= -n(\Lambda + \Delta) \prod_{i = 1}^n \br{1 + y_i^2 \ell''(y_i w^\top x_i)x_i^\top A_{i-1}^{-1}x_i}
    \end{aligned}
\end{equation}

We lower bound the ratio of determinant, 
\begin{equation}\label{eq:det-ratio-bound}
    \begin{aligned}
        \frac{\det\br{\nabla_wf(w; S_1')}^{-1}}{\det\br{\nabla_wf(w; S_2')}^{-1}} &= \frac{\det\br{\nabla_wf(w; S_2')}}{\det\br{\nabla_wf(w; S_1')}} \\
        &= \prod_{i = n/2 + 1}^n \frac{1+ \ell''(-w^\top x_i)x_i^\top A_{i-1}^{-1} x_i}{1+ \ell''(w^\top x_i)x_i^\top A_{i-1}^{-1} x_i} = 1
    \end{aligned}
\end{equation}
(DELTA)
where the last step follows from the property of the second derivative of logistic loss $\ell''(-z) = \ell''(z)$ as $\ell''(z) = \frac{1}{(1+e^{-z})(1+e^z)}$. 

Combining~\Cref{eq:one-to-one-function-w-to-b} and~\Cref{eq:det-ratio-bound} and choose $S$ such that $\lambda_n(XX^\top) \geq \Omega(\Lambda + \Delta)$ concludes the proof.  
\end{proof}

\begin{lem}[Matrix determinant lemma]\label{lem:matrix-determinant-lemma}
Let $\cA$ be an invertible square matrix of dimension $d$, and $u, v$ be two column vector of dimension $d$, then 
\[\det(A + uv^\top) = \det(A) \br{1 + v^\top A^{-1}u}\]

\end{lem}

Assume $z\in S$ is known. Let $b_x = \mathbbm{I}\{x\in S\}$ (randomness over the random coin $b$ in the membership game), $b_z^\pi = \mathbbm{I}\{z\in \pi(S \cup b_x\{x\})\}$ (randomness over $\pi$ given $S$, and $o$ be the random output of the algorithm $\cA(\pi(S))$.

\begin{lem}[Bayes rule of Entropy function]
Let $X, Y$ be two random variables, then
    \[H(Y|X) = H(X|Y) - H(X) + H(Y). \]
\end{lem}

 % Let $S' = S\setminus \{z\}$. Then, for deduplication we can express the distributions $P_0, P_1$. 
 % \begin{equation}
 % \begin{aligned}
 %          b_z^\pi &= 1 && b_x = 0\\
 %          &= b_\pi && b_x = 1
 % \end{aligned}
 % \end{equation}
 % Thus, 
 % \begin{equation}
 %     \begin{aligned}
 %         o &= \cA(\pi(S') \cup z) && b_x = 0\\
 %         &= \cA(\pi(S') \cup b_\pi z \cup (1-b_\pi) x) && b_x = 1
 %     \end{aligned}
 % \end{equation}

\begin{figure}
    \centering
    \begin{tikzpicture}
        % x node set with absolute coordinates
        % y node set relative to x.
        % Locations can be:
        % right,left,above,below,
        % above left,below right, etc
        \node[state] (x) at (0,0)  {$X$};
        \node[state] (xelse) [below =of x] {$X_{else}$};
        \node[state] (vpi1) [right =of x] {$V$};

        \node[state] (velse) [right =of xelse]{$W$};
        \node[state] (O) [right =of vpi1]{$O$};
        \node[state] (H) [below =of xelse] {$H$}; 
        
        % Directed edge

        \path (x) edge (vpi1); 
        \path (xelse) edge (vpi1); 
        \path (xelse) edge (velse); 
        \path (vpi1) edge (O); 
        \path (velse) edge (O); 
        \path (H) edge (vpi1); 
        \path (H) edge (velse); 

        % Bidirected edge
        % \path[bidirected] (x) edge[bend left=60] (y);
    \end{tikzpicture}
    \caption{Graph for Input dependent pre-processing}
    \label{graph:general-framework}
\end{figure}

\begin{itemize}
    \item $X$: a variable $X\in \{\cX, \emptyset\}$
    \item $X_{else}$: $X_{else}\in \cX^{n-1}$. The training set is defined as $S = X\cup X_{else}$. 
    \item $V$: variables that depends on $X$ after pre-processing
    \item $W$: variables that are independent of $X$ after pre-processing 
    \item $H$: abstract pre-processing variable
    \item $O$: output of the DP algorithm 
\end{itemize} 
\begin{proposition}
    Let $Z = \{V, W, H\}$ assuming $H$ is observable. Assume the support of $Z$ are discrete denote the support their index $supp(Z) = [m]$. Let $\pi$ be a pre-processing function that satisfies the conditional independence specified in~\Cref{graph:general-framework} and $\dpalg$ be an $(\epsilon, 0)$-DP algorithm, i.e. \begin{equation}
        \begin{aligned}
           V, W &= \pi(X\cup X_{else}, H), && V\perp W| X_{else}, H\\
            O &= \dpalg(V, W)
        \end{aligned}
    \end{equation}
    Then, we can get the following decomposition on the conditional likelihood ratio, for any $X_1\neq X_2\in \{\cX, \emptyset\}$, 
    \[ \frac{1}{m}\sum_{j = 1}^m \sqrt{r_{1, \min}^{(j)} r_{2, \min}^{(j)}} \leq \frac{\bP(O|X = X_1)}{\bP(O|X = X_2)}\leq \frac{1}{m}\sqrt{\br{\sum_{j = 1}^m r_{1, \max}^{(j)}}\br{\sum_{j = 1}^m r_{2, \max}^{(j)}}},\]
    where $r_{1, \max}^{(j)} = \max_{i \in [m]}\frac{\bP(O|Z = j)}{\bP(O|Z = i)} = \frac{1}{r_{1, \min}^{(j)}}$ and $r_{2, \max}^{(j)} = \max_{i \in [m]}\frac{\bP(Z = j|X = X_1)}{\bP(Z = i|X = X_2)} = \frac{1}{r_{2, \min}^{(j)}}$. 
\end{proposition}

\begin{proof}
    
\begin{equation}
    \begin{aligned}
        \frac{\bP(O|X = X_1)}{\bP(O|X = X_2)} &= \frac{\sum_{j = 1}^{[m]}\bP\br{O|Z = j}\bP\br{Z = j|X = X_1}}{\sum_{j = 1}^{[m]}\bP\br{O|Z = j}\bP\br{Z = j|X = X_2}}\\
        &= \sum_{j = 1}^{m} \br{\sum_{i = 1}^m \frac{\bP(O|Z = i)\bP(Z = i|X = X_1) }{{\bP(O|Z = j)\bP(Z = j|X = X_2) }}}^{-1}\\
        &\leq \frac{1}{m}\sum_{j = 1}^m \br{\min_{i \in [m]}\frac{\bP(O|Z = i) \bP(Z = i|X = X_1)}{\bP(O| Z = j) \bP(Z = j|X = X_2)}}^{-1}\\
        &\leq \frac{1}{m}\sum_{j = 1}^m \max_{i\in [m]}\frac{\bP(O|Z = j) \bP(Z = j|X = X_2)}{\bP(O| Z = i) \bP(Z = i|X = X_1)}\\
        &\leq \frac{1}{m}\sum_{j = 1}^m \br{\max_{i\in [m]}\frac{\bP(O| Z = j)}{\bP(O|Z = i)}}\br{\max_{i \in [m]}\frac{\bP(Z = j|X = X_1)}{\bP(Z = i|X = X_2)}}\\
        &\leq \frac{1}{m} \br{\sum_{j = 1}^m \max_{i\in [m]}\frac{\bP(O| Z = j)}{\bP(O|Z = i)}}^{\frac{1}{2}}\br{\sum_{j = 1}^m\max_{i \in [m]}\frac{\bP(Z = j|X = X_1)}{\bP(Z = i|X = X_2)}}^{\frac{1}{2}}j\\
        &= \frac{1}{m}\sqrt{\br{\sum_{j = 1}^m r_{1, \max}^{(j)}}\br{\sum_{j = 1}^m r_{2, \max}^{(j)}}}
    \end{aligned}
\end{equation}

Similarly, 
\begin{equation}
    \begin{aligned}
        \frac{\bP(O|X = X_1)}{\bP(O|X = X_2)} &= \frac{\sum_{j = 1}^{[m]}\bP\br{O|Z = j}\bP\br{Z = j|X = X_1}}{\sum_{j = 1}^{[m]}\bP\br{O|Z = j}\bP\br{Z = j|X = X_2}}\\
        &= \sum_{j = 1}^{m} \br{\sum_{i = 1}^m \frac{\bP(O|Z = i)\bP(Z = i|X = X_1) }{{\bP(O|Z = j)\bP(Z = j|X = X_2) }}}^{-1}\\
        &\geq \sum_{j = 1}^m \br{\sum_{i = 1}^m \frac{\bP(O|Z = i) }{\bP(O|Z = j)}}^{-\frac{1}{2}} \br{\sum_{i = 1}^m \frac{\bP(Z = i|X = X_1) }{\bP(Z = j|X = X_2)}}^{-\frac{1}{2}} \\
        &\geq \frac{1}{m}\sum_{j = 1}^m \br{\min_{i\in [m]} \frac{\bP(O|Z = j) }{\bP(O|Z = i)}}^{\frac{1}{2}}\br{\min_{i\in [m]} \frac{\bP(Z = j|X = X_2) }{\bP(Z = i|X = X_1)}}^{\frac{1}{2}} \\
        &= \frac{1}{m}\sum_{j = 1}^m \sqrt{r_{1, \min}^{(j)} r_{2, \min}^{(j)}}
    \end{aligned}
\end{equation}
\end{proof}

%     &\geq \sum_{j = 1}^m \br{\sum_{i=1}^m\frac{\bP(O|z = i)}{\bP(O|z = j)}}^{-1/2}\br{\sum_{i=1}^m\frac{\bP(z = i|b_1 = 0)}{\bP(z = j|b_1 = 1)}}^{-1/2} && \text{Cauchy Schwartz Inequality }\\
% &\geq \sum_{j = 1}^m \br{\max_{i \in [m]}\frac{m\bP(O|z = i)}{\bP(O|z = j)}}^{-1/2}\br{\max_{i \in [m]}\frac{m\bP(z = i|b_1 = 0)}{\bP(z = j|b_1 = 1)}}^{-1/2}\\
% &= \frac{1}{m}\sum_{j = 1}^m \br{\min_{i\in [m]}\frac{\bP(O|z = j)}{\bP(O|z = i)} }^{1/2}\br{\min_{i\in [m]}\frac{\bP(z = j|b_1 = 1)}{\bP(z = i|b_1 = 0)} }^{1/2}

\subsection{comparison with side channel}
\subsection{side information as MIA bit and reconstructed bit}

We define a pair of points $(x_i, x_j)$ to be $\alpha$-approximate duplicates if their distance $d(x_i, x_j)$ is less than some small threshold $\alpha$. Let the approximate deduplication algorithm $\pi_\alpha$ on a dataset $S$ be the procedure that randomly removes one point from each pair of $\alpha$-approximate duplicates in the dataset $S$ until no more duplicates can be found in $S$. 

\begin{figure}
    \centering
    \begin{tikzpicture}
        % x node set with absolute coordinates
        \node[state] (bx) at (0,0) {$b_x$};
        \node[state] (bpi) [below =of bx] {$b_\pi$}; 
    
        % y node set relative to x.
        % Locations can be:
        % right,left,above,below,
        % above left,below right, etc
        \node[state] (bz) [above =of bx] {$b_z$};
        \node[state] (bzpi) [right =of bx]{$b_z^\pi$};
        \node[state] (bxpi) [below =of bzpi]{$b_x^\pi$};
        \node[state] (O) [right =of bzpi]{$O$};
        % Directed edge
        \path (bx) edge (bzpi);
        \path (bz) edge (bzpi);  
        \path (bx) edge (bxpi); 
        \path (bz) edge (bxpi); 
        \path (bpi) edge (bxpi); 
        \path (bpi) edge (bzpi); 
        \path (bzpi) edge (O); 
        \path (bxpi) edge (O);
        
        % Bidirected edge
        % \path[bidirected] (x) edge[bend left=60] (y);
    \end{tikzpicture}
    \caption{Causal graph for deduplication (Full)}
    \label{fig:deduplication-causal-graph}
\end{figure}

\begin{thm}[Upper bound for privacy parameters with data deduplication]
    Let $\dpalg$ be an $(\epsilon, 0)$-DP algorithm. For any two neighboring datasets $S, S'$ differing exactly at the point $x$, i.e. $S' = S\cup\{x\}$. Assume $S, x$ satisfies that $d(x, x') \geq 2\alpha$ for all points $x'\in S$, and there exists a set $\{z_1, \ldots, z_{\ndedup}\}\subset S$ such that $d(z_i, x) \leq \alpha$ and $d(z_i, z_j) \geq \alpha$ for $i,j \in \{1,\ldots \ndedup\}$, then
    \[\max_{y\in \cO}\frac{\bP(\dpalg(\dedup(S)) \in y)}{\bP(\dpalg(\dedup(S'))\in y)}  \leq \frac{1}{2^{\ndedup}}e^{\ndedup\epsilon} + \br{1-\frac{1}{2^{\ndedup}}},\]
    where $\dedup(S)$ denotes data deduplication that randomly removes all but one points in each ball $B(x, \alpha)$, $x\in S$. 
\end{thm}

Note that the maximum value of $\ndedup$ depends on $\alpha$ and $d$. 

\begin{proof}
    Let $b_z, b_x$ denote the membership of the set of canaries $z$ and the target point $x$ in the original training set, $b_z^{\pi}$ be the randomness in the data-deduplication algorithm, $b_z^\pi, b_x^\pi$ be the membership of the set of canaries $z$ and the target point $x$ after de-duplication, and $O$ be the output of some $(\epsilon, \delta)$-DP algorithm. Then, we can define the variables with the causal graph \Cref{fig:deduplication-causal-graph} with the SCMs, 
    \begin{equation}
    \begin{aligned}
        b_x &= Ber(1/2) \\
        b_z &= 1\\
        b_z^\pi &= Ber\br{\frac{k-1}{k}}b_x + (1-b_x) = 1 - \br{1-Ber\br{\frac{k-1}{k}}}b_x\\
        b_x^\pi &= 1-b_z^\pi \\
        O &= \dpalg \br{\pi(S') \cup b_z^\pi \{z\} \cup b_x^\pi \{x\}}.
    \end{aligned}
    \end{equation}
    
By group privacy,
\begin{equation}
    \frac{\bP(O = y|b_z^\pi = 0)}{\bP(O = y|b_z^\pi = 1)}\leq e^{\ndedup\epsilon}.
\end{equation}

\begin{equation}
    \begin{aligned}
        \frac{\bP(O = y|b_x = 1)}{\bP(O = y|b_x = 0)} &= \frac{\frac{1}{\ndedup}\bP(O = y|b_z^\pi = 0) + \frac{\ndedup-1}{\ndedup}\bP(O = y|b_z^\pi = 1)}{\bP(O = y|b_z^\pi = 1)}\\
        &= \frac{1}{\ndedup}\frac{\bP(O = y|b_z^\pi = 0) }{\bP(O = y|b_z^\pi = 1) } + \frac{\ndedup-1}{\ndedup} \\
        &\leq \frac{1}{\ndedup}e^{\ndedup\epsilon} + \frac{\ndedup-1}{\ndedup} = e^{k'\epsilon}
    \end{aligned}
\end{equation}
where $k' = \frac{1}{\epsilon}\log\br{\frac{1}{\ndedup} e^{\ndedup\epsilon} + \frac{\ndedup-1}{\ndedup}}$. 

\end{proof}

Example where the upper bound is reached. Let $S = \{(X_i, 0)\}_{i = 1}^n$ such that $d(X_i, X_j)\geq \alpha$. Let $(x, 1)$ be a point such that $d(X_i, x)<\alpha$ for all $i\in [n]$. Let $f(S) = \sum_{i = 1}^n y_i$ and the $\epsilon$-DP algorithm $\cA_\epsilon$.  

% \begin{thm}[Lower bound for the privacy parameters with data deduplication]
%     Let $\dpalg$ be an $(\epsilon, 0)$-DP algorithm. For any two neighboring datasets $S, S'$ differing exactly at the point $x$, i.e. $S' = S\cup\{x\}$. Assume there exists a set $\{z_1, \ldots, z_{k_S}\}\subset S$ such that $d(z_i, x) \leq \alpha$ and $d(z_i, z_j) \geq \alpha$ for $i,j \in \{1,\ldots k_S\}$, then
%     \[\max_{y\in \cO}\frac{\bP(\dpalg(\pi(S)) \in y)}{\bP(\dpalg(\pi(S'))\in y)}  \geq \frac{1}{\ndedup}\br{1+ \sum_{i = 1}^{\ndedup}\frac{mem(\dpalg,S, z_i)}{\LOOAcc(\dpalg, S, z_i)}} + \frac{k_S-1}{k_S}\geq \frac{1}{\ndedup}\br{1 + \sum_{i = 1}^{\ndedup}mem(\dpalg, S, z_i) } + \frac{\ndedup - 1}{\ndedup},\]
%     where $\pi(S)$ denotes data deduplication that randomly removes all but one points in each ball $B(x, \alpha)$, $x\in S$. 
% \end{thm}

\begin{thm}[Upper bound for privacy parameters with mean imputation  ]
    Let $\dpalg$ be an $(\epsilon, 0)$-DP algorithm. For any two neighboring datasets $S, S'$ differing exactly at the point $x$, i.e. $S' = S\cup \{x\}$. Assume there exists a set $\{z_1, \ldots, z_{\nimput}\}\subset S$ where each point $z_i$ has at least one missing values on some features and $x$ does not have any missing value. Then, \[\max_{y\in  \cO}\frac{\bP\bs{\dpalg(\imput(S)) \in y}}{\bP\bs{\dpalg(\imput(S'))\in y}}\leq e^{\nimput \epsilon}. \]
\end{thm}
\begin{proof}
    Mean imputation can be expressed as the following graph with SCMs, 

\begin{figure}
    \centering
    \begin{tikzpicture}
        % x node set with absolute coordinates
        \node[state] (bx) at (0,0) {$b_x, X$};
        % y node set relative to x.
        % Locations can be:
        % right,left,above,below,
        % above left,below right, etc
        \node[state] (bz) [above =of bx] {$Z$};
        \node[state] (bzpi) [right =of bx]{$Z^\pi$};
        \node[state] (bxpi) [below =of bzpi]{$X^\pi$};
        \node[state] (O) [right =of bzpi]{$O$};
        % Directed edge
        \path (bx) edge (bzpi);
        \path (bz) edge (bzpi);  
        \path (bx) edge (bxpi); 
        \path (bzpi) edge (O); 
        \path (bxpi) edge (O);
        
        % Bidirected edge
        % \path[bidirected] (x) edge[bend left=60] (y);
    \end{tikzpicture}
    \caption{Causal graph for mean imputation (Full)}
    \label{fig:mean-imputation-causal-graph}
\end{figure}

    \begin{equation}
        \begin{aligned}
            X^\pi &= b_x X + (1-b_x) \emptyset \\
            Z^\pi &=( \imput(X\cup S) b_x + \imput (S) (1-b_x)), \\
            O &= \dpalg(Z^\pi) 
        \end{aligned}
    \end{equation}
    
    The proof follows directly by group privacy as data imputation where the target point has no missing value and at most $\nimput$ points have at least one missing values is deterministic. If $x$ is in the dataset, the two datasets after imputation differ at $\nimput$ points at most. 
\end{proof}

% \begin{thm}
%     Let $\cA$ be an $(\epsilon, 0)$-DP algorithm. For any two neighboring datasets $S, S'$ differing at the point $x$, i.e. $S' = S\cup \{x\}$. Assume $x$ does not have missing values and there are $k_S$ points $\{z_1, \ldots, z_{k_S}\}$ with missing values in $S$. Then, there exists a membership inference attack $\cA_{MIA}(S, x, \cA)$ with success rate \[\bP_b\bs{\hat{b} = b} \geq \sum_{\ell = k_S/2}^k \binom{k_S}{\ell}0.5^{k_S}(1+\gamma_i)^\ell(1 - \gamma_i)^{k_S
% -\ell}, \]
%     where $\gamma_i = mem(\cA, S, x_i)$ is the label memorization at point $x_i$. 
% \end{thm}
\begin{corollary}[Tighter upper bound for privacy parameters with mean imputation under strict privacy guarantee]
Let $S, S'$ be two neighboring datasets of size $n$ that differ at the point $x$ in the $d$-dimensional unit ball, i.e. $S' = S\cup \{x\}$. Under the following assumptions 
\begin{enumerate}
    \item There are $\nimput$ data points in $\{z_1, \ldots, z_{\nimput}\}\subset S$ with at least one missing values and $x$ has no missing value. 
    \item There exists a constant $n_{\min} \geq \nimput$ such that for every feature in the data, there are at least $n_{\min}$ data points in both $S$ and $S'$ where this feature is present and has a value (\ie it is not missing). 
    \item For $\epsilon, \delta > 0$, $\alpha > 1+\frac{\log \frac{1}{\delta}}{2\epsilon}$, let $\dpalg$ be an $(\alpha, \epsilon)$-RDP algorithm that has additive noise, \ie $\dpalg(S) = f(S) + g(Z)$, where $g$ is some arbitrary function over a random vector $Z$, and $f$ satisfies the following, there exists $\eta_1, \eta_2$ such that for all dataset $S$, $\forall z\in S$, $\norm{\frac{\partial f(z)}{\partial z}}\leq \eta_1$, $\norm{\frac{\partial^2 f(z)}{\partial z^2}}\leq \eta_2$, and $\max_{S\Delta S' = 1} \norm{f(S) - f(S')}_1 \geq \frac{\nimput\eta_1}{c n} + \br{\frac{\nimput \eta_2}{c n\sqrt{2}}}^2$. 
\end{enumerate}
 Then, $\dpalg\circ\pi$ is $(\br{(\ell+1)\epsilon}^{1.5}, \delta)$-DP, where \[\ell = \frac{\br{\frac{\nimput}{n_{\min}}\eta_1 + \br{\frac{\nimput}{\sqrt{2}n_{\min}}}^2\eta_2}}{\max_{S\Delta S' = 1}\norm{f(S) - f(S')}_1}.\] 
\end{corollary}

% \begin{proposition}[Tighter upper bound for privacy parameters with mean imputation for mechanisms with Gaussian noise]
% Let $S, S'$ be two neighboring datasets that differ at the point $x$, i.e. $S' = S\cup \{x\}$. Assume there are $\nimput$ data points in $\{z_1, \ldots, z_{\nimput}\}\subset S$ with at least one missing values and $x$ has no missing value. Denote the maximum sensitivity for mean imputation of $z_i$ by $\Delta_\mu$. Let $\dpalg$ be an $(\epsilon, 0)$ differential private algorithm with maximum variance $\sigma^2$. Assume the algorithm $\dpalg$ satisfies $\frac{\partial_S \dpalg(S)}{\partial S} = 0$ and $\norm{\frac{\partial^S \dpalg(S)}{\partial S^2}}_{op} \leq \eta$, For any $\alpha > 1$
% \[D_\alpha (\dpalg(\imput(S)||\dpalg(\imput (S')) \leq \frac{\alpha - \frac{1}{2}}{\alpha - 1}\Gamma(\sigma^2, \alpha, \Delta_\mu ) + \epsilon,\]
% where $D_\alpha(P||Q)$ denotes the $\alpha$-Renyi divergence between the distributions $P$ and $Q$ and $\Delta_\mu = \frac{1}{2}\norm{\pi(S)\cup \{x\} - \pi(S\cup \{x\})}^2 \eta$. 
% \end{proposition}
\begin{proof}
    Let $\pi_S$ be the data imputation with $S$ and $\pi_{S\cup \{x\}}$ be the data imputation with the set $S\cup \{x\}$. Let $D_1 = \pi_S(S)$ and $D_2 = \pi_{S\cup \{x\}}(S)$ and $D_3 = \pi_{S\cup \{x\}}(S\cup \{x\}) = \pi_{S\cup \{x\}}(S)\cup \{x\}$. Then, $D_2, D_3$ are neighboring datasets and $\norm{D_1 - D_2}^2 \leq \frac{\nimput}{cn}$.  
    
    Let $\Delta = D_2 - D_1$. As $f$ is smooth (Assump 3), by the error bound of Taylor expansion, 
    \begin{equation}
        \label{eq:smooth-assumption}
    \norm{f(D_2) -f(D_1)} - \frac{k_S\eta_1}{nc}       \leq  \norm{f(D_2) -f(D_1) -  \Delta^\top \frac{\partial f(D_1)}{\partial D_1}}_2 \leq \frac{1}{2}\Delta^\top \frac{\partial^2 f(D_1)}{\partial D_1^2} \Delta \leq \frac{1}{2}\br{\frac{k_S}{cn}}^2 \eta_2. 
    \end{equation}
    
    Thus, $f(D_2) + g(Z)$ and $f(D_1) + g(Z)$ satisfy the $(\alpha, \epsilon)$-RDP, which satisfies $(1.5\epsilon, \delta)$-DP for selected $\alpha = 1+\frac{\log \frac{1}{\delta}}{2\epsilon}$. Similarly, $f(D_2) + g(Z) $ and $f(D_3)+g(Z)$ also satisfy $(1.5\epsilon, \delta)$-DP. Then, we can conclude that $\dpalg\circ \pi$ is $(3\epsilon, \delta)$-DP by group privacy. 
\end{proof}

The previous corollary can be formulated with Fisher Information Loss: For a dataset $S$ and an algorithm $\dpalg$ with pdf of the output distribution $p_{\dpalg(S)}$, the FIL $I_n(S)$ is defined as \[I_n(S):= \norm{-\bE_{h\sim \dpalg(D)}\bs{\frac{\partial^2 \log p_{\dpalg(S)}(h)}{\partial S^2}}}_2,\]
where $\norm{\cdot}_2$ is the spectral norm. 

\begin{corollary}[Tighter upper bound for privacy parameters with mean imputation under strict privacy guarantee]
Let $S, S'$ be two neighboring datasets of size $n$ that differ at the point $x$ in the $d$-dimensional unit ball, i.e. $S' = S\cup \{x\}$. Under the following assumptions 
\begin{enumerate}
    \item There are $\nimput$ data points in $\{z_1, \ldots, z_{\nimput}\}\subset S$ with at least one missing values and $x$ has no missing value. 
    \item Let $c$ be some constant. For every feature in our data, there are at least $c n$ data points in both $S$ and $S'$ where this feature is present and has a value (\ie it is not missing). 
    \item For $\epsilon, \delta > 0$, $\alpha > 1+\frac{\log \frac{1}{\delta}}{2\epsilon}$, let $\dpalg$ be an $(\alpha, \epsilon)$-RDP algorithm that has additive noise, \ie $\dpalg(S) = f(S) + g(Z)$, where $g$ is some arbitrary function over a random vector $Z$, and $f$ satisfies the following, there exists $\eta$ such that for all dataset $S$, $I_n(S) \leq \eta$, and $\max_{S\Delta S' = 1} \norm{f(S) - f(S')}_1 \geq \exp\br{\frac{\eta\nimput}{nc}}-1$. 
\end{enumerate}
 Then, $\dpalg\circ\pi$ is $(3\epsilon, \delta)$-DP. 
\end{corollary}

Propose-Test-Release (PTR): test whether assumption 3 is satisfied and release the output only if assump 3 is satisfied. 

\begin{itemize}
    \item When PTR is combined with a specific DP-SGD on logistic regression, can we derive high probability guarantee on privacy? 
    \item Adapt existing DP algorithms to meet the smooth gradient requirement (regularization). 
\end{itemize}

\begin{defn}
    [Membership inference Game]
    
\end{defn}

\begin{thm}[Lower bound for privacy parameters for mean imputation]
    Let $\cA$ be an $(\epsilon, 0)$-DP algorithm. For any two neighboring datasets $S, S'$ differing at the point $x$, i.e. $S' = S\cup \{x\}$. Assume $x$ does not have missing values and there are $k_S$ points $\{z_1, \ldots, z_{k_S}\}$ with missing values in $S$. Then, there exists a membership inference attack $\cA_{MIA}(S, x, \cA)$ with success rate for the membership inference game defined above\[\bP_b\bs{\hat{b} = b} \geq \sum_{\ell = k_S/2}^k \binom{k_S}{\ell}p_i^\ell(1 - p_i)^{k_S
-\ell}\geq1 - \frac{p_i/2}{k_S\br{p_i - 1/2}^2},  \]
    where $p_i = 0.5 + 0.5\gamma_i$ and  $\gamma_i = mem(\cA, S, x_i)\leq e^\epsilon\LOOAcc(\cA, S, x)$ is the label memorization at point $x_i$. 
\end{thm}
\begin{proof}
    Assume that the attacker inserts $k$ canaries with $z^{(1)}, \ldots z^{(k)}$ with the $ith$ entry missing, $z^{(1)}_i = \ldots = z^{(k)}_i = NA$. If $x$ is not in the dataset, $z^{(1)}_i = \ldots = z^{(k)}_i = \bar{S}$, otherwise $z^{(1)}_i = \ldots = z^{(k)}_i = \overline{S\cup\{x\}}$. 
    
    Instead of membership inference, the attacker wants to infer the value of $z^{j}_i$ for all $j\in [k]$. Specifically, the attacker performs the following hypothesis test, $H_0^j: z^{(j)} = \bar{S}$ and $H_A^j:  z^{(j)} = \overline{S \cup \{x\}}$. Then, the attacker takes majority vote among the $k$ hypothesis testing. 

    We can lower bound the accuracy of a MIA test with an oracle to the label memorization (Feldman 20) of the DP algorithm. Assume the memorization at the point is at least $\gamma_i$, i.e. 
    \[mem(\cA, S, x_i) = \bP_{h\sim \cA(S)}\bs{h(x_i) = y} - \bP_{h\sim \cA(S^{\setminus x_i})}\bs{h(x_i) = y}\geq \gamma_i. \]

    In the following, we show that MIA as the likelihood ratio test with threshold $c = 1 + \min_{x_i\in S} mem(\cA, S, x_i)$ achieves accuracy $0.5 + 0.5\gamma_i$ at point $x_i$,  
    \begin{equation}
        \begin{aligned}
            acc(\psi(\cA, S, x_i)) &= \frac{1}{2}\bP_{y\sim P_0}\bs{\frac{P_0(y) }{P_1(y)}\geq c}+ \frac{1}{2}\bP_{y\sim P_1}\bs{\frac{P_0(y) }{P_1(y)}\leq  c}\\
            &= \frac{1}{2} + \frac{1}{2}\br{\bP_{y\sim P_0}\bs{\frac{P_0(y) }{P_1(y)}\geq c} - \bP_{y\sim P_1}\bs{\frac{P_0(y)}{P_1(y)}\geq c}}\\
            &= \frac{1}{2} + \frac{1}{2}\int_{y:\frac{P_0(y)}{P_1(y)}\geq c}P_0(y) - P_1(y)dy\\
            % &\geq \frac{1}{2} + \frac{1}{2}\int_{y:\frac{P_0(y)}{P_1(y)}\geq c}\br{c-1}P_1(y)
            & \geq \frac{1}{2} + \frac{1}{2}mem(\cA, S, x_i) \geq \frac{1}{2} + \frac{1}{2}\gamma_i
        \end{aligned}
    \end{equation}

    Then, the success rate of the majority vote of $k$ hypothesis tests can be viewed as the probability of $\bP(B \geq k/2)$ where $B$ is a binomial random varialbe with parameters $k$ and $0.5 + 0.5 \gamma_i$. The lower bound follows from the tail bound of binomial distributions. 
\end{proof}

% Take $c = e^\epsilon$, by the definition of approximate DP, \[\int_{y:\frac{P_0(y)}{P_1(y)}\geq e^\epsilon}P_1(y) = \bP_{z\sim PL(P_1||P_0)}\bs{z\geq \epsilon}\geq \delta'\]
% where $PL(P_1||P_0) = \log \frac{P_1(y)}{P_0(y)}$ is the privacy loss random variable with $y\sim P_1$. The last equality is by the assumption on the mechanism. For example, $\delta' = \phi\br{\frac{\sigma\epsilon}{\Delta} + \frac{\Delta}{2\sigma}} > 0 $ for Gaussian mechanism, where $\phi$ denotes the pdf of standard Gaussian distribution. 

Let $\Ak$ be the matrix whose columns consists of the eigenvectors corresponding to the first $k$ eigenvalues of SVD of $S$ and $\Akp$ be the matrix of top $k$ eigenvectors of SVD of $S\cup \{x\}$. Denote the $k^{th}$ and $k-1^{th}$ eigenvalue of the function by $\lambda_k$ and $\lambda_{k-1}$. 

\begin{thm}[Tighter upper bound for privacy parameters with PCA]
Let $S\in \cX^n$, $x\in \cX$ and $S' = S\cup \{x\}$. For any $\alpha > 1$, let $\dpalg$ be an $(\alpha, \epsilon)$-RDP algorithm that has additive noise, $\dpalg(S) = f(S) + g(Z)$, where $g$ is arbitrary function over a random vector $Z$ and $f$ satisfies the following, there exists $\eta$ such that for all dataset $S$, $\norm{\frac{\partial f(z)}{\partial z}}\leq \eta_1$ and $\norm{\frac{\partial^2f(z)}{\partial z^2}}\leq \eta_2$ and $\max_{S\Delta S' = 1} \norm{f(S) - f(S')}_1 \geq \frac{\eta_1}{\lambda_k - \lambda_{k-1}} + \frac{\lambda_2}{2(\lambda_k - \lambda_{k-1})^2}$. Then, $\cA\circ\pi_{pca}$ is $(\alpha, 3\epsilon)$-RDP.
\end{thm}

\begin{proof}
    By Theorem 3 in Zwald05, as all $x\in \cX$ satisfies $\norm{x}_2\leq 1$, \[\norm{\Akp\Akp^\top - \Ak\Ak^\top}\leq \frac{1}{(n+1)(\lambda_k - \lambda_{k-1})}\]
    Thus, 
    \begin{equation}\label{eq:pca-convergence-subspace}
        \norm{\Akp\Akp^\top S - \Ak\Ak^\top S} \leq \norm{\Akp\Akp^\top - \Ak\Ak^\top}\norm{S} \leq \frac{n}{(n+1)(\lambda_k - \lambda_{k-1})}.
    \end{equation}
    Let $D_1 = \Akp S$, $D_0 = \Ak S$ and $D_2 = \Akp S'$. We note that $D_1, D_2$ are neighboring datasets, and $D_0, D_1$ satisfies $\norm{D_0 - D_1} \leq \frac{n}{(n+1)(\lambda_k - \lambda_{k-1})}$ by~\Cref{eq:pca-convergence-subspace}. 

    From the smoothness assumption of the function $f$, 
      \begin{equation}        \label{eq:pca-smooth-assumption}
      \begin{aligned}
          \abs{f(D_0) -f(D_1)} - \frac{\eta_1}{\lambda_{k}-\lambda_{k-1}}  & \leq  \abs{f(D_0) -f(D_1) -  (D_0 - D_1)^\top \frac{\partial f(D_1)}{\partial D_1}}_2 \\
          &\leq \frac{1}{2}(D_0 - D_1)^\top \frac{\partial^2 f(D_1)}{\partial D_1^2} (D_0 - D_1) \\
          &\leq \frac{\eta_2}{2(\lambda_k - \lambda_{k-1})}. 
      \end{aligned}
    \end{equation}
    Rearrange \Cref{eq:pca-smooth-assumption}, for $D_0, D_1$ obtained with any $S, S'$, 
    \begin{equation}
        \label{eq:pca-sensitivity-condition}
        \abs{f(D_0)-f(D_1)}\leq \frac{\eta_1}{\lambda_k - \lambda_{k-1}} + \frac{\eta_2}{2(\lambda_k - \lambda_{k-1})^2}\leq \max_{S\Delta S' = 1}\abs{f(S) - f(S')}. 
    \end{equation}
\end{proof}

\begin{thm}
    Let $S, S'$ be any two neighboring datasets differing at the point $x$. Let $\Ak, \Akp$ be the projection matrix consisting of the first $k$ eigenvectors of $Cov(S)$ and $Cov(S')$ respectively. Denote $\cS_{c_1, c_2}$ be the set of neighboring datasets such that $\Ak, \Akp$ satisfies $\Ak - \Akp \leq c_1 xx^\top + c_2 \br{xx^\top}^{\perp}$, \ie \[\cS_{c_1, c_2}= \{(S, S'): S\Delta S' = x, \Ak\ - \Akp \leq c_1 xx^\top + c_2 \br{xx^\top}^{\perp}\}.\]
     \[\cS_{c_1, c_2}= \{(S, S'): S\Delta S' = x, \Pi_{xx^\top}\br{\Ak\ - \Akp} \leq c_1~\mathrm{and}~\br{\bI - \Pi_{xx^\top}}\br{\Ak\ - \Akp} \leq c_2 \}.\]
    Let $\cA$ be an $(\epsilon, \delta)$- DP algorithm that successfully minimizes empirical loss $\nabla_\theta E_{\theta\sim \cA(S)}( \ell(\theta, S)) = 0$ and low Fisher Information Loss (FIL) $\eta$ on each training point, then 
    \[\max_{(S, S')\in \cS_{c_1, c_2}}\max_{O \in \cH}\frac{\bP\bs{\cA(\Ak S) \in O}}{\bP\bs{\cA(\Akp S') \in O}}\leq f(\epsilon, \delta, \eta, c_1, c_2). \]
\end{thm}

First order derivative of the parameters upper bounded by $\epsilon, \delta$, and second order derivative of the parameters should be upper bounded by FIL $\eta$. 

\begin{proof}
% \begin{lem}\label{eq:lem1}
%     Let $\cA$ be an $(\epsilon, \delta)$-DP algorithm, then \[\bE_{h_S\sim \cA(S)} \bs{\frac{\partial h_S}{\partial S}}\leq f_1(\epsilon, \delta) = n\epsilon_i,\] 
%     where $\epsilon_i$ represents the individual privacy parameter of point $x_i$. 
% \end{lem}

Denote $\Ak - \Akp = \Delta_{S, S'} \leq C(c_1, c_2)$. Then, \[\Akp S' = \begin{pmatrix}
    \Ak S + \Delta_{S, S'} S\\
    \Ak x + \Delta_{S, S'} x
\end{pmatrix} = 
    \Ak S' + \Delta_{S, S'} S'.
    \]

\begin{equation}
    \begin{aligned}
        \bE [\cA(\Akp S')] &= \bE[\cA(\Ak S' + \Delta_{S, S'} S')]\\
        &\approx \bE[\cA(\Ak S' )]+ \frac{\partial\bE[\cA(\Ak S')]}{\partial S'}\Delta_{S, S'} S' + \frac{\partial^2\bE[\cA(\Ak S')]}{2\partial (S')^2}\br{\Delta_{S, S'} S' }^2\\
        &\leq \bE[\cA(\Ak S' )]+ \frac{\partial \bE[\cA(\Ak S')]}{\partial \theta}\frac{\partial \theta}{\partial S'}\Delta_{S, S'}S' + \frac{\eta}{2}C(c_1, c_2)^2 \\
        &= \bE[\cA(\Ak S' )]+ \frac{\eta}{2}C(c_1, c_2)^2 
    \end{aligned}
\end{equation}
We can then bound the mean divergence between $\cA(\Akp S') $ and $\cA(\Ak S)$ with a function of $\epsilon, \delta, \eta, C(c_1, c_2)$. 

\end{proof}

\paragraph{Minimizing the smooth DP parameter for DP-ERM through regularization} 

Let $B(x, r) = \{x': d(x', x) \leq r\}$ be the ball with radius $r$ and origin $x$. 
\begin{lem}
    Given two functions $f, g$ that are Lipschitz continuous with paramter $L_1, L_2$ respectively. Let the objective function $F = \gamma_1 f + \gamma_2g$ for some fixed parameter $\gamma_1, \gamma_2$. Let $\theta_f^\star = \argmin_{\theta\in \Theta} f(\theta)$ and $\theta_g^\star = \argmin_{\theta\in \Theta} g(\theta)$. 
    Then, gradient descent for $T$ steps with learning rate $\eta$ on $F$ satisfies 
    \begin{align*}
        f(\theta_T) - f(\theta_f^{\star}) &\leq c_1 + \frac{\norm{\theta_0 - \theta_{F}^\star}}{2\gamma_1\eta T}\\
        g(\theta_T) - g(\theta_f^{\star}) &\leq c_2 + \frac{\norm{\theta_0 - \theta_{F}^\star}}{2\gamma_2 \eta T},
    \end{align*}
    where $c_1 = f(\theta_{f+g}^\star)- f(\theta_f^\star)$ and $c_2 = g(\theta_{f+g}^\star) - g(\theta_g^\star)$. 
\end{lem}
\begin{proof}
    Following the standard analysis of the convergence bound of gradient descent, we have 
    \begin{equation}
        \label{eq:lem-gd-convergence-bound}
        F(\theta_T) - F(\theta_{g+f}^\star)\leq \frac{\norm{\theta_0 - \theta_F^*}}{2\eta T}.
    \end{equation}
    Note that both $f(\theta_T) - f(\theta_F^\star)$ and $g(\theta_T) - g(\theta_F^\star)$ are non-negative. By \cref{eq:lem-gd-convergence-bound}, 
    \begin{equation}
        \label{eq:lem-seperate-convergence-bound}
        \begin{aligned}
            f(\theta_T) - f(\theta_F^\star)&\leq \frac{\norm{\theta_0 - \theta_F^*}}{2\gamma_1\eta T}\\
             g(\theta_T) - g(\theta_F^\star)&\leq \frac{\norm{\theta_0 - \theta_F^*}}{2\gamma_2\eta T}. 
        \end{aligned}
    \end{equation}
    We can break the left hand side of \cref{eq:lem-seperate-convergence-bound} with two parts $\br{f(\theta_T) - f(\theta_f^\star)}$ and $ \br{f(\theta_f^\star)-f(\theta_F^\star)}$. Rearranging the second components, we can establish the first inequality. Repeat the procedure for the function $g$ concludes the proof. 
\end{proof}

Assume $f, g$ are $\sigma$-strongly convex. Denote the event that the minimizer of the sum of the objective function resides in the ball around $\theta_f^\star$ ( Kuwaranancharoen 23)\[\cE = \left\{\min_{\theta\in B\br{\theta_f^\star, \frac{\gamma_1^2 L_1^2}{\sigma}}} F(\theta) \leq \min_{\theta\in B\br{\theta_f^\star, \frac{\gamma_2^2L_2^2}{\sigma}}} F(\theta)\right\}\]
Then $c_1 \leq \mathbbm{1}\{E\}\norm{\theta_f^\star - \theta_g^\star}+\frac{\gamma_1L_1^2}{\sigma}$ and $c_2 \leq \norm{\theta_f^\star - \theta_g^\star}\br{1-\mathbbm{1}\{E\}} + \frac{\gamma_2L_2^2}{\sigma}$. 

Choose $\gamma_1 = \frac{1}{n}$ and $T = O(n^2)$, then 
\[ f(\theta_T) - f(\theta_f^{\star}) \leq \mathbbm{1}\{E\}\norm{\theta_f^\star - \theta_g^\star}+\frac{L_1^2}{n\sigma} + \frac{\norm{\theta_0 - \theta_{F}^\star}}{2\gamma_1\eta n}.\]

Approximate method for linear models: regularization $\norm{\theta}_2$?
