# Supplementary material for: Provable Privacy with Non-Private Pre-Processing
Source: arXiv:2403.13041 source file (2024-06-21)
Supplement: Supplementary file 2 [file linear-projectionMIA.tex]

We define the membership inference game as follows 
\begin{defn}[Single round MIA Game with pre-processing]\label{defn:MIA-game-projection}
    Given a training set $S = (X, Y) \in (\cX\times \cY)^n$ and a point of inference $z = (x, y)$, define a single round of MIA game as follows, \begin{enumerate}
        \item The attacker runs an projection generation algorithm $\cA_{pre}(S, z)$ that takes as input the training set $S$ and the point of inference $z$ and output a projection matrix $\Pi$. 
        \item The model trainer  runs a $(\epsilon, \delta)$-DP algorithm $\dpalg$ to calculate $\theta_1 \leftarrow \dpalg(S)$ and $\theta_2 \leftarrow \dpalg(X\Pi\cup\{ \Pi^\top x\}, Y\cup\{y\})$. Then, the model trainer tosses a coin $b\sim Ber(1/2)$ and outputs $\thetahat \leftarrow (1-b)\theta_1 + b \theta_2$. 
        \item The attacker runs the MIA algorithm $\hat{b} \leftarrow \algMIA(\Pi, S, z, \thetahat)$ that takes as input the information that is available and outputs a guess on $b$.  
    \end{enumerate}
\end{defn}

In the following, we instantiate the MIA game defined in~\Cref{defn:MIA-game-projection} with a specific set of projection matrices $\Pi$, a specific DP algorithm $\cA_{exp}$ and MIA algorithm defined $\algMIA$ defined below. 

{\color{red}remove the constraint on projection matrix and add the step to normalize $X$ before calculating the loss; sample $d\sim Ber(1/2), \theta_3 = \dpalg(\pi_2(S_1(x_2, y_2))$, output $b\theta_1 + (1-b)d\theta_2 + (1-b)(1-d)\theta_3$ }
\begin{algorithm}
\caption{$\cA_{exp}$: Exponential sampling with convex loss functions (Bassily14)}\label{alg:exponential-mechanism-for-erm}
\textbf{Input}: a training set $S$ of size $n$, a $L$-Lipschitz convex loss function $\ell: \cC \times (\cX\times \cY)\rightarrow \reals_+$, privacy parameter $\epsilon$, a convex set $\cC$
    \begin{algorithmic}[1]
        \State Let $\cL(\theta; S) = \sum_{i = 1}^n \ell(\theta; (x_i, y_i))$ for $\theta\in \cC$. 
        \State Define the distribution $D_\epsilon$ over $\cC$ with PDF $f_\epsilon(\theta) = \frac{1}{Z} \exp\br{-\frac{\epsilon \cL(\theta; S)}{2Ln \norm{\cC}_2}}$, where $Z = \int_\cC \exp\br{-\frac{\epsilon \cL(\theta; S)}{2Ln \norm{\cC}_2}} d\theta$. 
        \State Output $\thetahat \sim D_\epsilon$. 
    \end{algorithmic}
\end{algorithm}

\begin{algorithm}
\caption{$\algMIA^\gamma$: MIA attack with loss threshold $\gamma$}
\textbf{Input}: a projection matrix $\pi$, a training set $S = (X, Y)$ and a point of inference $z = (x, y)$, output of the DP algorithm $\cA_{exp}$ $\thetahat$, and the $L$-Lipschitz loss function $\ell$ used in $\cA_{exp}$
\begin{algorithmic}[1]
    \State Let $\Gamma(\Pi, \thetahat, S, z) = \frac{1}{n}\cL(\thetahat; S) - \frac{1}{n+1}\cL(\thetahat; (X\Pi, Y)\cup \{(\Pi^\top x, y)\})$
    \State output $\hat{b} = \mathbbm{1}\{\Gamma(\Pi, \thetahat, S, z)\geq \gamma\}$
\end{algorithmic}
\end{algorithm}

\begin{thm}
    Assume that the adversary can only choose a projection matrix $\Pi$ that approximately preserves the length of  $x\in X\cup \{x\}$ and $\theta \in \cC$ and exactly preserves the true signal $\theta^\star$, 
    \begin{equation}
        \label{assumpt:rip-projection-matrices}
        (1-\zeta)x^\top \theta \leq x^\top \Pi \Pi^\top \theta\leq (1+\zeta)x^\top \theta, \quad \norm{\Pi^\top \theta^\star} = \norm{\theta^\star}.
    \end{equation}
    Let the DP algorithm be $\cA_{exp}$ with square loss and the MIA algorithm be $\algMIA^\gamma$, then the success rate of the adversary is upper and lower bounded by \begin{equation}
       \bP_{\tilde{\theta}\sim \cN\br{\br{v_{\min} - \frac{1}{n+1}I_{n+1}}Y_2, v_{\min}v_{\min}^\top \frac{2Ln\norm{\cC}_2}{\epsilon}}}\bs{\norm{\tilde{\theta}}^2\geq \gamma}\leq  TPR \leq \bP_{\tilde{\theta}\sim \cN\br{\br{v_{\max} - \frac{1}{n+1}I_{n+1}}Y_2, v_{\max}v_{\max}^\top \frac{2Ln\norm{\cC}_2}{\epsilon}}}\bs{\norm{\tilde{\theta}}^2\geq \gamma}
    \end{equation}
where $v_{\max} = \begin{pmatrix}
\br{\frac{1}{(1-\zeta)^2 n} - \frac{1}{n+1}} I_n \\-\frac{1}{n+1}[0, \ldots, 1]
\end{pmatrix}$ and $v_{\min} = \begin{pmatrix}
\br{\frac{1}{(1+\zeta)^2 n} - \frac{1}{n+1}} I_n \\-\frac{1}{n+1}[0, \ldots, 1]
\end{pmatrix}$. 
\end{thm}

\begin{equation}
       TPR = O\br{\frac{L\norm{\cC}_2}{(1-\zeta)^4n\epsilon\gamma}}
    \end{equation}
\begin{proof}
    Write $S_2 = \br{\begin{pmatrix}
        X\\x^\top
    \end{pmatrix}, \begin{pmatrix}Y\\y\end{pmatrix}} = \br{X_2, Y_2}$. Then, the true positive rate of the MIA can be written as 
    \begin{equation}
        \label{eq:def-TPR}
        TPR = \bP\bs{\algMIA(S, z, \Pi, \dpalg) = 1|b = 1}
    \end{equation}
    According to \Cref{alg:exponential-mechanism-for-erm}, the PDF of the output distribution of $\theta$ when $b = 1$ can be written as 
    \begin{equation}
        f_{\epsilon}(\theta) = \frac{1}{Z}\exp\br{-\frac{\epsilon \norm{X_2\Pi\Pi^\top\theta - Y_2}^2}{2L\norm{\cC}_2n}},
    \end{equation}
    which indicates that \Cref{alg:exponential-mechanism-for-erm} is identical as sampling $X_2\Pi\Pi^\top\theta$ from the $\cN\br{Y_2, \frac{2Ln\norm{\cC}_2}{\epsilon}I_{n+1}}$. Thus, 
    \begin{equation}
        \label{eq:deriv-TPR1}
    \begin{aligned}
        TPR 
        &= \bP_{X_2\Pi\Pi^\top \theta\sim \cN\br{Y_2, \frac{2Ln\norm{\cC}_2}{\epsilon}I_{n+1}}}\bs{\Gamma(\theta, \Pi, S, z)\geq \gamma}\\
        &= \bP_{\theta\sim \cN\br{ZY_2, \frac{2Ln\norm{\cC}_2}{\epsilon}ZZ^\top}}\bs{\Gamma(\theta, \Pi, S, z)\geq \gamma},
    \end{aligned}
\end{equation}
where $Z = \br{X_2\Pi\Pi^\top}^{-1}$. 

Next, we rewrite $\Gamma$ with the notation of $X_2$ and $\tilde{X}_2$, 
\begin{equation}\label{eq:def-gamma}
    \Gamma(\Pi, \theta, S, z) = \frac{1}{n}\norm{X\theta - Y}^2 - \frac{1}{n+1}\norm{X\Pi\Pi^\top \theta - Y}^2 - \frac{1}{n+1}(x^\top \Pi\Pi^\top \theta - y)^2
\end{equation}

Then, we rewrite the second term in \Cref{eq:def-gamma} to derive upper and lower bound of $\Gamma$, \begin{equation}\label{eq:loss-in-projection-space}
    \begin{aligned}
        \norm{X\Pi^\top \theta - Y}^2 &= \norm{X\Pi\Pi^\top \theta - X\theta^\star}^2\\
        &= \norm{X\br{\Pi\Pi^\top \theta -\Pi\Pi^\top \theta^\star + \Pi\Pi^\top \theta^\star - \theta^\star}}\\
        &= \norm{X\br{\Pi\Pi^\top}\br{\theta - \theta^\star}} 
    \end{aligned}
\end{equation}
where the last equation follows from the second assumption on the projection matrix in~\Cref{assumpt:rip-projection-matrices}. 

By the first assumption (RIP) in~\Cref{assumpt:rip-projection-matrices}, we can bound the loss in the original space with the loss in the projection space 
\begin{equation}\label{eq:loss-bounds}
    \frac{1}{(1+\zeta)^2}\norm{X\Pi\Pi^\top \theta - Y}^2 \leq \norm{X\theta - Y}^2 \leq \frac{1}{(1-\zeta)^2}\norm{X\Pi\Pi^\top \theta - Y}^2 
\end{equation}

Substituting \Cref{eq:loss-bounds} into \Cref{eq:def-gamma}, we have the following bounds on $\Gamma$, \begin{equation}
    \label{eq:bounds-from-rip}
    \begin{aligned}
        \Gamma(\Pi, \theta, S, z) &\geq \br{\frac{1}{(1+\zeta)^2 n} - \frac{1}{n+1}}\norm{X\Pi\Pi^\top \theta - Y}^2 - \frac{1}{n + 1}(x^\top \Pi\Pi^\top - y)^2 = \norm{v_{\min}X_2\Pi\Pi^\top \theta - Y_2}^2\\
        \Gamma(\Pi, \theta, S, z) &\leq \br{\frac{1}{(1-\zeta)^2 n} - \frac{1}{n+1}}\norm{X\Pi\Pi^\top \theta - Y}^2 - \frac{1}{n + 1}(x^\top \Pi\Pi^\top - y)^2 = \norm{v_{\max}X_2\Pi\Pi^\top \theta - Y_2}^2
    \end{aligned}
\end{equation}

where $v_{\min} = \begin{pmatrix}
    \br{\frac{1}{(1+\zeta)^2n} - \frac{1}{n+1}}I_{n}\\-\frac{1}{n+1}[0, \ldots, 1]
\end{pmatrix} = \begin{pmatrix}
    \frac{1}{(1+\zeta)^2n} - \frac{1}{n+1}&0&\ldots &0&0\\
    0&\frac{1}{(1+\zeta)^2n} - \frac{1}{n+1}&\ldots&0&0\\
    0&0&\ldots &\frac{1}{(1+\zeta)^2n} - \frac{1}{n+1}&0\\
    0&0&\ldots &0&-\frac{1}{n+1}
\end{pmatrix}$ and $v_{\max} = \begin{pmatrix}
    \br{\frac{1}{(1-\zeta)^2n} - \frac{1}{n+1}}I_{n}\\-\frac{1}{n+1}[0, \ldots, 1]
\end{pmatrix} = \begin{pmatrix}
    \frac{1}{(1-\zeta)^2n} - \frac{1}{n+1}&0&\ldots &0&0\\
    0&\frac{1}{(1-\zeta)^2n} - \frac{1}{n+1}&\ldots&0&0\\
    0&0&\ldots &\frac{1}{(1-\zeta)^2n} - \frac{1}{n+1}&0\\
    0&0&\ldots &0&-\frac{1}{n+1}
\end{pmatrix}$. 

Then, we can write the upper and lower bound of the true positive rate of the proposed simple MIA as 
\begin{equation}\label{eq:mia-tpr-upper-bound}
    \begin{aligned}
        TPR &\leq \bP_{\theta\sim \cN\br{ZY_2, \frac{2Ln\norm{C}_2}{\epsilon}ZZ^\top}} \bs{\norm{v_{\max}X_2\Pi\Pi^\top \theta - Y_2}^2\geq \gamma} \\
        &= \bP_{\tilde{\theta}\sim \cN\br{\br{v_{\max} - \frac{1}{n+1}I_{n+1}}Y_2, v_{\max}v_{\max}^\top \frac{2Ln\norm{\cC}_2}{\epsilon}}}\bs{\norm{\tilde{\theta}}^2\geq \gamma}\\
        TPR &\geq \bP_{\theta\sim \cN\br{ZY_2, \frac{2Ln\norm{C}_2}{\epsilon}ZZ^\top}} \bs{\norm{v_{\max}X_2\Pi\Pi^\top\theta - Y_2}^2\geq \gamma}\\
        &= \bP_{\tilde{\theta}\sim \cN\br{\br{v_{\min} - \frac{1}{n +1}I_{n+1}}Y_2, v_{\min}v_{\min}^\top \frac{2Ln\norm{\cC}_2}{\epsilon}}}\bs{\norm{\tilde{\theta}}^2\geq \gamma}
    \end{aligned}
\end{equation}
where the distribution of $\tilde{\theta}$ are generalized chi-square distribution. 
\end{proof}

We can write the variance in the upper and lower bound
\begin{equation}
\begin{aligned}
       &v_{\min}v_{\min}^\top \frac{2Ln\norm{\cC}_2}{\epsilon} =  \\& \begin{pmatrix}2Ln\norm{\cC}_2\br{\frac{1}{(1+\zeta)^2n} - \frac{1}{n+1}}^2&0&\ldots &0&0\\
    0&2Ln\norm{\cC}_2\br{\frac{1}{(1+\zeta)^2n} - \frac{1}{n+1}}^2&\ldots&0&0\\
    0&0&\ldots &2Ln\norm{\cC}_2\br{\frac{1}{(1+\zeta)^2n} - \frac{1}{n+1}}^2&0\\
    0&0&\ldots &0&\frac{2Ln\norm{\cC}_2}{\br{n+1}^2}
\end{pmatrix}
\end{aligned}
\end{equation}
and 
\begin{equation}
\begin{aligned}
       &v_{\max}v_{\max}^\top \frac{2Ln\norm{\cC}_2}{\epsilon} = \\&\begin{pmatrix} 2Ln\norm{\cC}_2\br{\frac{1}{(1-\zeta)^2n} - \frac{1}{n+1}}^2&0&\ldots &0&0\\
    0&2Ln\norm{\cC}_2\br{\frac{1}{(1-\zeta)^2n} - \frac{1}{n+1}}^2&\ldots&0&0\\
    0&0&\ldots &2Ln\norm{\cC}_2\br{\frac{1}{(1-\zeta)^2n} - \frac{1}{n+1}}^2&0\\
    0&0&\ldots &0&\frac{2Ln\norm{\cC}_2}{\br{n+1}^2}
\end{pmatrix} 
\end{aligned}
\end{equation}

\section{general framework with KL divergence}

 Let $P_0$ denote the output distribution when $x$ in the training set and $P_1$ denote the output distribution when $x$ is not in the training set.

Let $O$ represent the random output of the DP algorithm. 
 \begin{equation}\label{eq:kl-decomposition}
     \begin{aligned}
         KL(O, b_z^\pi|b_x = 0|| O, b_z^\pi|b_x = 1) &= KL(P_0(O, b_z^\pi)||P_1(O, b_z^\pi) ) \\
         &= \bE_{b_z^\pi\sim P_{0, b_z^\pi}}KL(P_0(O|b_z^\pi)||P_1(O|b_z^\pi) ) + \sum_{O\in \cY}\sum_{b_z^\pi}P_0(O, b_z^\pi) \log\frac{P_0(b_z^\pi)}{P_1(b_z^\pi)}\\
         &= \bE_{b_z^\pi\sim P_{0, b_z^\pi}}KL(P_0(O|b_z^\pi)||P_1(O|b_z^\pi) ) + \sum_{b_z^\pi}P_0(b_z^\pi) \log\frac{P_0(b_z^\pi)}{P_1(b_z^\pi)}\\
         &= \bE_{b_z^\pi\sim P_{0, b_z^\pi}}KL(P_0(O|b_z^\pi)||P_1(O|b_z^\pi) ) + KL(P_{0, b_z^\pi}||P_{1, b_z^\pi})
     \end{aligned}
 \end{equation}

For binary tests $\psi_S: \cY\times \{0, 1\}\rightarrow \{0, 1\}$ that returns the membership of $x$ given an output, $b_z^\pi$ pair. 
\begin{equation}\label{eq:lecam-inequality}
    \begin{aligned}
        \frac{1}{2}\bP\bs{\psi_S(O_S, b_z^\pi) \neq b_x} &= \frac{1}{2}\br{1-\norm{P_{0}(O_S, b_z^\pi) - P_1(O_S, b_z^\pi)}_{TV}}\\
        &\geq \frac{1}{2}\br{1-\sqrt{\frac{1}{2}KL(P_0(O_S, b_z^\pi||P_1(O_S, b_z^\pi)}}\\
        &= \frac{1}{2}\br{1-\sqrt{\frac{1}{2}\br{\bE_{b_z^\pi\sim P_{0, b_z^\pi}}KL(P_0(O|b_z^\pi)||P_1(O|b_z^\pi) ) + KL(P_{0, b_z^\pi}||P_{1, b_z^\pi})}}}
    \end{aligned}
\end{equation}
where the last equality follows from~\Cref{eq:kl-decomposition}. i.e.
\begin{equation}
    \bP\bs{\psi_S(O_S, b_z^\pi) \neq b_x} \geq \frac{1}{2}\br{1-\sqrt{\frac{1}{2}\br{\bE_{b_z^\pi\sim P_{0, b_z^\pi}}KL(P_0(O|b_z^\pi)||P_1(O|b_z^\pi) ) + KL(P_{0, b_z^\pi}||P_{1, b_z^\pi})}}}
\end{equation}

The upper bound can be attained by analysing the Neyman-Pearson test $\psi_S^{NP}$. By Theorem 9 in \cite{1055254}, 
\begin{equation}
    \max\{P_0\bs{\psi_S^{NP}(O_S, b_z^\pi) \neq 1}, P_1\bs{\psi_S^{NP}(O_S, b_z^\pi) \neq 0}\} \leq \max\{e^{-r}, e^{-e(r)}\}
\end{equation}
where $e(r) = \min_{P\in \cP_r} KL(P||P_1)$, where $\cP_r = \{P: KL(P, P_0)\leq r\}$. 

The following lower bound on KL divergence holds, 
%(https://people.lids.mit.edu/yp/homepage/data/LN_fdiv.pdf)
\begin{equation}
    KL(P||P_1)\leq \frac{2\log e}{\min_x P_1(x)} TV(P, P1)
\end{equation}
Let the set $\cP_r^{TV} = \{P: \frac{2\log e}{\min_x P_1(x)} TV(P, P1)\leq r\}$, then $\cP_r\subset \cP_r^{TV}$. 

Then, we can derive an lower bound on $e^{-e(r)}$, 
\begin{equation}
    \begin{aligned}
        e(r) &= \min_{P \in \cP_r} KL(P||P_1) \\
            &\geq \min_{P\in \cP_r^{TV}}KL(P||P_1)&& \text{By}\cP_r\subset \cP_r^{TV} \\
            &\geq \min_{P\in \cP_r^{TV}} 2TV(P, P_1)^2\\
            &\geq \min_{P\in \cP_r^{TV}} 2\br{TV(P_0, P_1) - TV(P_0, P)}^2\\
            &\geq \left\{ \begin{array}{ll}
         2TV(P_0, P_1)^2 & \mbox{if $TV(P_0, P_1)\leq r$};\\
        2(TV(P_0, P_1) - r)^2 & \mbox{if $TV(P_0, P_1) > r$}.\end{array} \right.\\
        &\geq \left\{ \begin{array}{ll}
         \frac{\br{\min_xP_1(x)}^2}{2\log^2 e}KL(P_0, P_1)^2 & \mbox{if $TV(P_0, P_1)\leq r$};\\
        2\br{\frac{\min_x P_1(x)}{2\log e}KL(P_0, P_1) - r}^2 & \mbox{if $TV(P_0, P_1) > r$}.\end{array} \right.
    \end{aligned}
\end{equation}

% If $P_0, P_1$ are both Gaussian distributions and all $P\in \cP_r$ are restricted to Gaussian distributions, a weak form of triangle inequality holds for their $KL$ divergence \cite{zhang2023properties}. Then, we can derive an upper bound for the error of Neyman Pearson test, \begin{equation}
% \begin{aligned}
%         &\max\{P_0\bs{\psi_S^{NP}(O_S, b_z^\pi) \neq 1}, P_1\bs{\psi_S^{NP}(O_S, b_z^\pi) \neq 0}\} \\
%         \leq& \max\left\{\exp(-r), \exp(-3(r+\bE_{b_z^\pi\sim P_{0, b_z^\pi}}KL(P_0(O|b_z^\pi)||P_1(O|b_z^\pi) ) + KL(P_{0, b_z^\pi}||P_{1, b_z^\pi})))\right\}
% \end{aligned}
% \end{equation}

 %  \begin{equation}
 %     I(b_x; o, b_z^\pi) = I(b_x; o) - I(b_z^\pi; b_x|o).
 % \end{equation}

 % \begin{equation}
 %     \begin{aligned}
 %         I(b_x; o, b_z^\pi) &= H(b_x) - H(b_x|o, b_z^\pi) \\
 %         &= H(b_x) - H(b_z^\pi|b_x, o) + H(b_z^\pi|o) - H(b_x|o) && \text{Bayes rule}\\
 %         &= I(b_x; o) - H(o|b_x, b_z^\pi) + H(o|b_x) - H(b_z^\pi|b_x) + H(b_z^\pi|o)   &&\text{Bayes Rule}\\
 %        &= I(b_x; o) - H(b_z^\pi|o, b_x) + H(b_z^\pi|b_x) - H(o|b_x) + H(o|b_x) - H(b_z^\pi|b_x) + H(b_z^\pi|o) \\
 %        &= I(b_x; o) - H(b_z^\pi|o, b_x) + H(b_z^\pi|o) \\
 %        &= I(b_x; o) + I(b_z^\pi, b_x|o) 
 %     \end{aligned}
 % \end{equation}
 % Here $I(b_x; o; b_z^\pi)$ is positive by the definition of $b_z^\pi$ and $o$. 
