# Supplementary material for: Provable Privacy with Non-Private Pre-Processing
Source: arXiv:2403.13041 source file (2024-06-21)
Supplement: Supplementary file 3 [file non-private-PCA.tex]

Let $S = \{(x_i, y_i)\}_{i = 1}^n$ and $S' = S\cup \{(x, y)\}$ be two neighboring datasets. 

Let $\pi_k$ be the non-private PCA, i.e. first $k$ components of $S$ if $(x_1, x_2)$ is not in the dataset, and first $k$ components of $S'$ if $(x, y)$ is in the dataset. 

\begin{thm}\label{thm:pca}
    Let $\cA$ be the obejctive perturbation with regularized cross-entropy loss, $L(w; S) = \frac{1}{n}\sum_{i = 1}^n \ell(w; (x_i, y_i)) + \frac{\Lambda}{2}\norm{w}_2^2$ with $c = 1/4$ and $\pi_k$ be non-private PCA with $k$ components. Then, the following statements hold simultaneously, 
    \begin{itemize}
        \item $\cA$ is $(\epsilon, 0)$-DP on the projected $k$-dimensional space,
        \item $\cA$ is $(\epsilon_1(n), 0)$-DP on the original data space,
        \item $\max_{S, S', o}\log \br{\frac{\bP\bs{\cA(\pi_k(S))\in o}}{\bP\bs{\cA(\pi_k(S'))\in o}}}\geq \Omega (\epsilon_2(n))$. 
    \end{itemize}
\end{thm}

\begin{proof}
    For fixed $S = (X, Y)$, $X^T X = U\Lambda U^T$ with $\Delta_k = \lambda_{k} - \lambda_{k+1}\leq \delta$ denoting the difference between the $k$th eigenvalue and the $k+1$th eigenvalue and $U = [u_1, \ldots u_d]$ denoting the corresponding eigenvectors. Choose $x = u_{k+1}$. Let $\delta \leq \frac{1}{n+1}\norm{x}_2$, then \begin{equation}
        \pi_k (\tilde{x}) = \begin{cases} 
      \begin{pmatrix}
          u_1^\top \tilde{x} &
          \ldots 
          u_{k-1}^\top\tilde{x} &
          u_k^\top \tilde{x}
      \end{pmatrix}^\top  & (x, y)\in S \\
       \begin{pmatrix}
          u_1^\top \tilde{x} &
          \ldots&
          u_{k-1}^\top\tilde{x} &
          u_{k+1}^\top \tilde{x}
      \end{pmatrix}^\top & \text{otherwise}
   \end{cases}
    \end{equation}
    Similar to the proof of~\Cref{thm:deduplication}, we write \begin{equation}
        \begin{aligned}
            \tilde{S} &= 
        \end{aligned}
    \end{equation}

    \begin{equation}
        \begin{aligned}
            \frac{\bP[\cA(\pi(S)) = w]}{\bP[\cA(\pi(S')) = w]}
            &=         \frac{\bP[\cA(S) = w]}{\bP[\cA(S') = w]}\\
            &= \frac{\bP[b = f(w, S_1')]\abs{\text{det}(\nabla_w f(w; S_1'))}^{-1}}{\bP[b = f(w, S_2')]\abs{\text{det}(\nabla_w f(w; S_2'))}^{-1}} 
        \end{aligned}
    \end{equation}
\end{proof}
